# Supplementary material for: A central limit theorem for the matching number of a sparse random graph
Source: arXiv:2402.05851 ancillary file (2025-01-26)
Supplement: Supplementary file 1 [file computations.pdf]

## Initial fluctuations (for Lemma 4.3)

$$\text{In}[1]:= \text{pi}[j\_] := E^{-c} c^j / j!$$

$$\text{In}[2]:= \text{cov}[j\_ , k\_ ] := \text{pi}[j] \times \text{pi}[k] \left( \frac{(j-c)(k-c)}{c} - 1 \right)$$

$$\text{In}[3]:= \Sigma_{1,1} = \text{cov}[1, 1] + \text{pi}[1];$$

$$\Sigma_{1,2} = \Sigma_{2,1} = \text{Sum}[\text{cov}[1, k], \{k, 2, \infty\}];$$

$$\Sigma_{1,3} = \Sigma_{3,1} = \text{Sum}[(k/2) \text{cov}[1, k], \{k, 0, \infty\}] + \text{pi}[1]/2;$$

$$\Sigma_{2,2} = \text{Sum}[\text{cov}[j, k], \{j, 2, \infty\}, \{k, 2, \infty\}] + \text{Sum}[\text{pi}[j], \{j, 2, \infty\}];$$

$$\Sigma_{2,3} = \Sigma_{3,2} = \text{Sum}[(k/2) \text{cov}[j, k], \{j, 2, \infty\}, \{k, 0, \infty\}] + \text{Sum}[(j/2) \text{pi}[j], \{j, 2, \infty\}];$$

$$\Sigma_{3,3} = \text{Sum}[(j/2)(k/2) \text{cov}[j, k], \{j, 0, \infty\}, \{k, 0, \infty\}] + \text{Sum}[(j/2)^2 \text{pi}[j], \{j, 0, \infty\}];$$

$$\text{In}[9]:= \text{Table}[\Sigma_{i,j}, \{i, 3\}, \{j, 3\}] // \text{Simplify} // \text{MatrixForm}$$

Out[9]//MatrixForm=

$$\begin{pmatrix} c e^{-2c} (1 - 3c + c^2 + e^c) & -c e^{-2c} (-1 - 2c + c^2 + e^c) & -((-1+c) c e^{-c}) \\ -c e^{-2c} (-1 - 2c + c^2 + e^c) & e^{-2c} (-1 - c^2 + c^3 + e^c + c(-2 + e^c)) & c^2 e^{-c} \\ -((-1+c) c e^{-c}) & c^2 e^{-c} & \frac{c}{2} \end{pmatrix}$$

## Estimating the fluid limit (for Section 5.1)

$$\text{In}[10]:= \text{f}[u\_ ] := E^u - u - 1$$

$$\text{In}[11]:= \text{F}_1[x1\_ , x2\_ , x3\_ ] := -1 - \frac{x1}{2 x3} + \frac{x2^2 z[x1, x2, x3]^4 E^{z[x1, x2, x3]}}{(2 x3 \text{f}[z[x1, x2, x3]])^2} - \frac{x1 x2 z[x1, x2, x3]^2 E^{z[x1, x2, x3]}}{(2 x3)^2 \text{f}[z[x1, x2, x3] ]};$$

$$\text{F}_2[x1\_ , x2\_ , x3\_ ] := -1 + \frac{x1}{2 x3} - \frac{x2^2 z[x1, x2, x3]^4 E^{z[x1, x2, x3]}}{(2 x3 \text{f}[z[x1, x2, x3]])^2};$$

$$\text{F}_3[x1\_ , x2\_ , x3\_ ] := -1 - \frac{x2 z[x1, x2, x3]^2 E^{z[x1, x2, x3]}}{2 x3 \text{f}[z[x1, x2, x3] ]};$$

$$\text{In}[14]:= \beta[z\_ ] := \text{ProductLog}[c E^z] / c$$

(The Mathematica command for the Lambert W function is "ProductLog".)

$$\text{In}[15]:= \text{chi}_1[z\_ ] := \frac{1}{c} (z^2 - z c \beta[z] (1 - E^{-z}));$$

$$\text{chi}_2[z\_ ] := (1 - (1 + z) E^{-z}) \beta[z];$$

$$\text{chi}_3[z\_ ] := \frac{1}{2c} z^2;$$

Now, let's re-express the drift function in terms of z:

```
In[18]:= F[z_] := {F1[x1, x2, x3], F2[x1, x2, x3], F3[x1, x2, x3]} /.
  {z[x1, x2, x3] -> z, x1 -> chi1[z], x2 -> chi2[z], x3 -> chi3[z]}
```

Let's do a series expansion (Fact 5.2):

```
In[19]:= Series[F[z], {z, 0, 0}] // MatrixForm
```

Out[19]//MatrixForm=

$$\begin{pmatrix} 2(-1 + \text{ProductLog}[c]^2) + O[z]^1 \\ (-\text{ProductLog}[c] - \text{ProductLog}[c]^2) + O[z]^1 \\ (-1 - \text{ProductLog}[c]) + O[z]^1 \end{pmatrix}$$

## Computing $\partial F$ (for Lemma 5.3)

We will need to use implicit differentiation to compute  $\partial z / \partial x_i$ , so we introduce a quantity  $Q$ , which according to the definition of  $z$  can be expressed either in terms of  $z$  or  $x$ .

```
In[20]:= Q[z_] := \frac{(-1 + e^z) z}{f[z]}
```

```
Q[x1_, x2_, x3_] := \frac{-x1 + 2 x3}{x2}
```

(Note that  $\partial z / \partial x_i = \partial Q / \partial x_i \cdot dz / dQ$ , and  $dz / dQ$  is the reciprocal of  $Q'[z]$ .)

```
In[22]:= dF = Table[
  D[Fi[x1, x2, x3], xj] /.
  {z^(1,0,0)[x1, x2, x3] -> Q^(1,0,0)[x1, x2, x3] / Q'[z[x1, x2, x3]],
  z^(0,1,0)[x1, x2, x3] -> Q^(0,1,0)[x1, x2, x3] / Q'[z[x1, x2, x3]],
  z^(0,0,1)[x1, x2, x3] -> Q^(0,0,1)[x1, x2, x3] / Q'[z[x1, x2, x3]],
  z[x1, x2, x3] -> z, x1 -> chi1[z], x2 -> chi2[z], x3 -> chi3[z]},
  {i, 3}, {j, 3}];
```

Now let's rewrite in terms of  $z$ , and do a series expansion around zero.

```
In[23]:= Series[dF /. {z[x1, x2, x3] -> z, x1 -> chi1[z], x2 -> chi2[z], x3 -> chi3[z]}, {z, 0, -2}] /.
  {ProductLog -> W} // MatrixForm
```

Out[23]//MatrixForm=

$$\begin{pmatrix} \frac{3c-7cW[c]}{z^2} + \frac{1}{O[z]} & -\frac{6(-c+cW[c])}{z^2} + \frac{1}{O[z]} & -\frac{2(3c-7cW[c]+4cW[c]^2)}{z^2} + \frac{1}{O[z]} \\ \frac{c+2cW[c]}{z^2} + \frac{1}{O[z]} & \frac{1}{O[z]} & \frac{2(-c-cW[c]+2cW[c]^2)}{z^2} + \frac{1}{O[z]} \\ \frac{4c}{z^2} + \frac{1}{O[z]} & \frac{6c}{z^2} + \frac{1}{O[z]} & \frac{-8c+2cW[c]}{z^2} + \frac{1}{O[z]} \end{pmatrix}$$

Next we want to diagonalise this matrix for Lemma 5.3. Let's first rescale by  $z^2$  and get rid of the error terms.

```
In[24]:= H = Limit[z^2 %, z -> 0];
```

In[25]:= **H // Eigenvectors // Transpose // MatrixForm**

Out[25]//MatrixForm=

$$\begin{pmatrix} -2(-1+W[c]) & \frac{1}{2}(1-4W[c]+3W[c]^2) & -4W[c] \\ W[c] & \frac{1}{2}(1+W[c]-2W[c]^2) & 1+2W[c] \\ 1 & 1 & 1 \end{pmatrix}$$

(This is the matrix Q in Lemma 5.3.)

In[26]:= **DiagonalMatrix[H // Eigenvalues] // MatrixForm**

Out[26]//MatrixForm=

$$\begin{pmatrix} 0 & 0 & 0 \\ 0 & -3c(1+W[c]) & 0 \\ 0 & 0 & -2c(1+W[c]) \end{pmatrix}$$

(This is the matrix D in Lemma 5.3.)
